# Supplementary material for: Risk-Aware Linear Bandits: Theory and Applications in Smart Order Routing
Source: arXiv:2208.02389 source file (2026-04-02)
Supplement: Supplementary file 1 [file appendix_contextual.tex]

\section{Extension: Risk-aware Contextual Bandit} \label{sec:contextual}
In many financial applications such as smart order routing, market-making, and intra-day trading, the reward (e.g., profit-and-loss) depends on the real-time market microstructure such as order flow imbalance and  volatility \citep{cont2014price,hambly2021recent}. Motivated by this practical consideration, this section considers the framework of \textit{contextual bandit} where a random context arrives at each time point, representing the current market condition in the financial applications. The unknown coefficients in the model depend on the realization of the context. 
 
Mathematically, we assume that the context $Z_t$ arrives at the beginning of each round $t$ and they are $i.i.d.$  following a categorical distribution $\operatorname{CG} \paren{\bfp} = [p_1, \cdots, p_M]$, which we call the \textit{arrival distribution}. 
Upon observing $Z_t = c$, we assume that the reward follows
$$X_t = \inner{ A_t, \theta_{*}^c } + \eta_t(A_t), \quad\text{with}$$ 
\begin{align} \label{eq:var_def_context}
 \eta_t(A_t) \sim \mathcal{N} \left (0, f( \inner{ \phi_{*}^{c}, A_t  } ) \right), \quad
f(\inner{ \phi_{*}^{c}, A_t  }) = \inner{ \phi_{*}^{c}, A_t  } + \omega ,
\end{align}
where  $\omega$ is some constant which ensures the variance is non-negative. Here vectors $\theta_{*}^{c}, \phi_{*}^{c} \in \mathbb{R}^d$ are unknown parameters with bounded $\ell_2$-norm, \textit{i.e.}, $\| \theta_{*}^c \|_2 \leq 1 , \| \phi_{*}^c \|_2 \leq \omega  ,$ so that $ f( \inner{ \phi_{*}^c, A_t  } ) \in [\sigma_{\min}^2, \sigma_{\max}^2]$. In addition, we assume the  action set $\mathcal{A}$ is fixed over time regardless of the current context.

In the presence of contexts, the benchmark policy $\pi^*$ is the one that has the knowledge of $\braces{\theta_*^c}_{c=1}^{M}, \braces{\phi_*^c}_{c=1}^{M}$ and selects the best action with the smallest mean-variance given the context. 
Namely, given $Z_t=c$, then the best action $a_t^*$ is the one which attains the best mean-variance, i.e. $a_t^* = \argmin_{a \in \mathcal{A}}  \inner{\phi_*^c , a }  - \rho \inner{ \theta_*^c, a}  $ .

\begin{algorithm}[htbp]
  \caption{The Contextual Risk-Aware Explore-then-Commit (\crise) Algorithm.} \label{algo:contextualExpExp}
\begin{algorithmic}[]
\small 
\State (1) Given $\mathcal{A}$, find the $G$-optimal design $Q^*$ as the solution to  % \eqref{eq:g-optimal} 
\begin{align}
    \nonumber&\underset{Q(\cdot)}{\operatorname{minimize}} ~g(Q):=\max_{a\in\cA}a^{\top}\left(\sum_{a\in\cA}Q(a)aa^{\top}\right)^{-1}a\\
    \label{eq:g-optimal}&\text{s.t.,}~\sum_{a\in\cA}Q(a)=1\,,\ Q(a)\geq 0~~~\forall a\in\cA.  \nonumber 
\end{align}
% so that $Q^*$ has at most $ d(d+1) / 2$ non-zero entries.
\State (2) For the first $n=d T^{2/3}$ rounds, observe the current context $c$. Select the next action in $N_{(c)}$. 
\State (3) Compute least squares estimates for each $c \in [M]$ % \eqref{eq:theta_estimate_MV} and \eqref{eq:phi_estimate_MV}.
\begin{align}
    &\hat{\theta}_n^{(c)} = \paren{\sum_{s=1}^{n} \one{Z_s=c} X_sX_s^\top }^{-1} \sum_{s=1}^{n} \one{Z_s=c} X_s A_s, \nonumber  \\
    &\hat{\phi}_{n}^{(c)} = \paren{\sum_{s=1}^{n} \one{Z_s=c} X_sX_s^\top }^{-1} \sum_{s=1}^{n} \one{Z_s=c}  f^{-1} \left( \left ( X_s - \inner{\hat{\theta}_{n}^{(c)} , \,A_s} \right )^2 \right) A_s \ . \nonumber 
\end{align}
\State (4) For the remaining $T - n$ rounds, select the action that maximizes the estimated MV
$$
 \hat{a}^*_t = \arg \min_{a \in \mathcal{A}} \inner{  \hat{\phi}_n^{(Z_t)} -\rho \hat{\theta}_n^{(Z_t)} \ ,a}  \ . 
$$ % following \eqref{eq:a_star}.

\end{algorithmic}
\end{algorithm}

We propose the Contextual Risk-Aware Explore-then-Commit (\crise) Algorithm.
It is a variant to the \rise~algorithm, distinguished by a core modification that adapts to the random arrival of contexts.
Note that in the contextual case, we lack the luxury of freely selecting actions as in the noncontextual scenario discussed in Sections \ref{sec:formulation}-\ref{sec:risepp}. Consequently, we must plan ahead and adjust the estimation tolerance based on the anticipated number of context arrivals.
To be specific, we find the $G$-optimal design $Q^*$ as the solution to Step (1) in Algorithm~\ref{algo:contextualExpExp}. 
Then in Step (2), for each context $c$, we set the estimation tolerance $\varepsilon_{(c)} = \frac{\sqrt{2}}{\sqrt{p_c}} \tilde{C} \sqrt{\log d \log^2\paren{MT}} d T^{-\frac{1}{3}}$.
This way, we will explore more according to the $G$-optimal design for the more frequently seen contexts. 
We let the set of actions (repetitions allowed) to be explored under context $c$ be $N_{(c)}$, with $n_{(c)}^{a} = \left \lceil  \frac{ \tilde{C}^2 d^3 \log{(d)}\log^2 \left( MT\right)  Q^* (a)  }{\varepsilon_{(c)}^2}   \right \rceil$ many action $a$ in it. 
When it comes to the exploitation phase, we use the samples collected in the exploration phase to estimate the coefficients of each context individually. 
Specifically, in Step (4), whenever the context is $c$, we will select the actions one by one in the set $N_{(c)}$.

\begin{proposition} \label{prop:temporal_decomposition_context}
Given the knowledge of the arrival distribution $[p_1, \cdots, p_M]$, 
the expected regret of policy $\crise$ is bounded by $\tilde{\Theta} \paren{ d T^{\frac{2}{3}} \sqrt{M} }$. 

% \begin{equation}
%    \E{\reg_\pi(T)} =  \E{ \sum_{t=1}^{T} \inner{\phi_* - \rho \theta_*, A_{t}^{\pi} - a_t^* } } 
%    + \E{ \sum_{t=1}^{T-1}  \frac{1}{ (t+1)}  \sum_{s=1}^{t} \left( \inner{\theta_*, A_{t+1}^{\pi} - A_{s}^{\pi} } \right)^2 }  
%    + O\paren{\sqrt{T}}  \ .   \label{eq:expected_regret_upper_bound_sqrtT_context}
% \end{equation}    
\end{proposition}
The key idea in this proof replies on adapting the decomposition method from Proposition~\ref{prop:temporal_decomposition} to the contextual case. 
The formal proof can be found in \ref{prop:temporal_decomposition_context}. 

To this end, we denote by $\mu_*$ the random mean of the actions taken by the single-arm optimal policy and $\sigma_*^2 $ the random variance of the actions taken by the single-arm optimal policy. 
Let $*(j)$ be the index of the best action in terms of MV given that the context is $j$. 
Hence, we have $\E{ \mu_* } = \sum_{j=1}^{M} p_j \mu_{*(j)}  $ and $\E{ \sigma_*^2 }  = \sum_{j=1}^{M} p_j  \sigma_{*(j)}^2 $. 

We need to first show that the variance of rewards over $T$ periods of the optimal policy $\E{ \sum_{t=1}^{T}  \paren{ X_t^* - \E{ \mu_* } }^2 }$ is lower bounded by $T \sum_{j=1}^{M} p_j  \sigma_{*(j)}^2  = T \E{ \sigma_*^2 }$. 
Given this, we can now apply the decomposition and divide contexts into two groups: frequent contexts and rare contexts.
In the presence of random contexts, the estimation error in the exploitation phase can be still properly controlled, even though we have no control over the frequency in which we see a particular context. 
This is because, due to the $i.i.d.$ arrival, we can expect to encounter contexts that were extensively explored during the exploration phase with a high degree of frequency in the exploitation phase, and vice versa.  For frequent contexts, we can achieve a reliable estimation. However, for rare contexts, our estimations might be somewhat coarse due to limited data, but their contribution to the overall regret is also minimal.

\subsection{Proof of Proposition~\ref{prop:temporal_decomposition_context}}

% We denote by $\mu_*$ the random mean of the actions taken by the single-arm optimal policy and $\sigma_*^2 $ the random variance of the actions taken by the single-arm optimal policy. 
% Let $*(j)$ be the index of the best action in terms of MV given that the context is $j$. 
% Hence, we have $\E{ \mu_* } = \sum_{j=1}^{M} p_j \mu_{*(j)}  $ and $\E{ \sigma_*^2 }  = \sum_{j=1}^{M} p_j  \sigma_{*(j)}^2 $. 

To proceed, we first show that the variance of rewards over $T$ periods of the optimal policy $\E{ \sum_{t=1}^{T}  \paren{ X_t^* - \E{ \mu_* } }^2 }$ is lower bounded by $T \sum_{j=1}^{M} p_j  \sigma_{*(j)}^2  = T \E{ \sigma_*^2 }$. 
Indeed, we note that 
\begin{eqnarray*}
    & &  \E{ \sum_{t=1}^{T}  \paren{ X_t^* - \E{ \mu_* } }^2 }  \\ 
    &=&  \sum_{t=1}^{T} \sum_{j=1}^{M} p_j \E{  \paren{ X_t^* - \E{ \mu_* } }^2 \mid Z_t = j}  \\ 
    &=& T \sum_{j=1}^{M} p_j  \E{ \paren{X_t^* }^2  +  \paren{ \E{ \mu_* } }^2 - 2 X_t^* \E{ \mu_* } \mid Z_t = j  }   \\ 
    &=& T \sum_{j=1}^{M} p_j \paren{ \sigma_{*(j)}^2 + \mu_{*(j)}^2  +  \paren{\E{ \mu_* } }^2  - 2 \mu_{*(j)} \E{ \mu_* }  }  \\ 
    &=&   T \sum_{j=1}^{M} p_j  \sigma_{*(j)}^2 + T  \paren{ \sum_{j=1}^{M} p_j  \mu_{*(j)}^2 - \paren{ \sum_{j=1}^{M} p_j  \mu_{*(j)} }^2 }   \\ 
    &\geq&  T \sum_{j=1}^{M} p_j  \sigma_{*(j)}^2  = T \E{ \sigma_*^2 } \ , 
\end{eqnarray*}
where the last inequality follows since $ \paren{\sum_{j=1}^{M} p_j  \mu_{*(j)}}^2 \leq \paren{ \sum_{j=1}^{M} p_j } \paren{ \sum_{j=1}^{M} p_j \mu_{*(j)}^2}  $.

Given this observation, we are now ready to invoke the same reasoning to upper bound the expected regret as Proposition~\ref{prop:temporal_decomposition}. 
First, following the same calculation as in \eqref{eq:per_round_regret_decomposition_1}, the instantaneous regret of policy $\pi$ can be bounded by 
\begin{equation}  \label{eq:upper_bound_three_terms_context}
     \E{ r_\pi(t+1)}  \leq \E{  \frac{1}{t(t+1)} \left( t X_{t+1}^{\pi} - \sum_{s=1}^{t} X_{t}^{\pi} \right)^2 - \rho X_{t+1}^{\pi} } - \paren{  \E{ \sigma_*^2 } - \rho \E{ \mu_* } }  \ . 
\nonumber
\end{equation}
Now, continuing with the same rationale as expressed in \eqref{eq:decomposition_final_eq}, we obtain that 
\begin{equation} \label{eq:context_regret_bound}
   \E{\reg_\pi(T)} \leq  \E{ \sum_{t=1}^{T} \inner{\phi_* - \rho \theta_*, A_{t}^{\pi} - a_t^* } } 
    + \E{ \sum_{t=1}^{T-1}  \frac{1}{ (t+1)}  \sum_{s=1}^{t} \left( \inner{\theta_*, A_{t+1}^{\pi} - A_{s}^{\pi} } \right)^2 }  
    + O\paren{\sqrt{T}} \ .   
\end{equation}
We proceed to deal with the first two terms in the sequel.
\begin{enumerate}
    \item 
Let $\tau^{\operatorname{exp}}_{i, c }$ and $ \tau^{\operatorname{cmt}}_{i, c }$ be the number of times that action $i$ is selected when under context $c$ during the exploration phase and exploitation phase, respectively. Similarly,
let $\tau_{\cdot, c}^{\operatorname{exp}}$ and $ \tau^{\operatorname{cmt}}_{\cdot, c }$ be the number of times that context $c$ shows up in the exploration phase and exploitation phase, respectively. 

To proceed, we state a concentration result of multinomial distribution. 
\begin{lemma}[Lemma 5 in \cite{kawaguchi2022robustness}] \label{lemma:multinomial_bound}
If $X_1, X_2, \cdots, X_M$ are multinomially distributed with parameters $n$ and $p_1, \cdots, p_M$, then for any $\delta > 0$, with probability at least $1- \delta$, the following holds for all $i \in [M]$: 
\begin{equation}
    p_i - \frac{X_i}{n} \leq \sqrt{\frac{2 p_i \ln \paren{M / \delta}}{n}}  \ . \nonumber 
\end{equation}
\end{lemma}

Denote by $n$ the length of exploration phase, and we set it to be $n = d T^{\frac{2}{3}}$. 
Let $F = \{ c \in [M] :  p_c > \frac{8 \ln \paren{MT} }{n} \}$ be the set of indices of frequently seen contexts.  
Note that depending on the problem instance, the cardinality of set $F$ can range from 0 to $M$. 
Invoking Lemma~\ref{lemma:multinomial_bound}, we know that with probability at least $1-\frac{1}{T}$, it holds for all $c \in [M]$ that 
\begin{equation}  \label{eq:multinomial_bound_context}
    \tau_{\cdot, c}^{\operatorname{exp}} \geq p_c n - \sqrt{2 p_c n \ln \paren{ MT }} \ .
\end{equation}
Recall that $x \geq \frac{b}{a - \theta}$ satisfies the quadratic inequality $a x^2 - b x \geq \theta x^2 $ where $a > \theta > 0 $ and $b > 0$. 
Hence, if $\sqrt{n} \geq \frac{\sqrt{2 p_c \ln \paren{MT}}}{p_c - \frac{1}{2} p_c}$, then $\tau_{\cdot, c}^{\operatorname{exp}} \geq p_c n - \sqrt{2 p_c n \ln \paren{ MT }} \geq \frac{1}{2 } p_c n$. 
Consequently, for any frequent context $c \in F$, 
we will observe these contexts frequently often compared to their expected number of arrivals. 
Namely, it holds that $ \tau_{\cdot, c}^{\operatorname{exp}} \geq \frac{1}{2} p_c n $. 

When \eqref{eq:multinomial_bound_context} happens, according to Proposition~\ref{prop:bound_ip}, we can characterize the estimation error of the G-optimal design exploration: 
\begin{equation} \label{eq:estimation_error_bound_context}
    \p{ \left | \inner{a, \phi_{*}^c - \rho \theta_{*}^c} - \inner{a, \hat{\phi}_{n}^c - \rho \hat{\theta}_{n}^c  } \right | \leq \varepsilon_{(c)} ,~~\forall~a \in \mathcal{A} ,  ~ \forall~c \in F  } \geq 1 - \frac{1}{T} \ , 
\end{equation}
by setting $\varepsilon_{(c)} = \frac{\sqrt{2}}{\sqrt{p_c}} \tilde{C} \sqrt{\log d \log^2\paren{MT}} d T^{-\frac{1}{3}}$ in \crise. 
%\Renyuan{explain why and especially the cardinality of $F$.}
%\Jingwei{This is simply an application of Proposition 1, just like in the previous section. I think the point of this design here is that we do not need to worry about the cardinality of $F$ too much, either it be small (0) or large ($M$). The point is that we adjust the estimation error according to its expected arrival times.  }

For frequent contexts in $F$, when the event in \eqref{eq:estimation_error_bound_context} happens, since we take actions greedily with respect to $\inner{a, \hat{\phi}_{n}^c - \rho \hat{\theta}_{n}^c  } $, we have $\inner{\phi_* - \rho \theta_*, A_{t}^{\pi} - a_t^* }  \leq  2 \varepsilon_{(c)} $. 
When the event in \eqref{eq:estimation_error_bound_context} does not happen, we bound $\inner{\phi_* - \rho \theta_*, A_{t}^{\pi} - a_t^* }$ simply by $2  \paren{ \sigma_{\max}^{2} - \sigma_{\min}^{2} + 2 \rho}$.
Hence, we obtain 
\begin{eqnarray*}
& & \E{ \sum_{t=n+1}^{T} \inner{\phi_* - \rho \theta_*, A_{t}^{\pi} - a_t^* } }   \\ 
&\leq&  \sum_{t=n+1}^{T} \paren{ \sum_{ c \in F } p_c 2 \varepsilon_{(c)} + \sum_{c \in F^\complement} 2 p_c \paren{ \sigma_{\max}^{2} - \sigma_{\min}^{2} + 2 \rho}  }  
+ \sum_{t=n+1}^{T} \frac{2}{T} \cdot 2 \paren{ \sigma_{\max}^{2} - \sigma_{\min}^{2} + 2 \rho}  \\
  &=&  \tilde{\Theta} \paren{ (T-n) d T^{-\frac{1}{3}} \sum_{c \in F} \sqrt{p_c}   
  + \paren{ T-n } \sum_{c \in F^{\complement}  } d^{-1} T^{-\frac{2}{3}}   }  \\
  &\leq&  \tilde{\Theta} \paren{ d T^{\frac{2}{3}} \sqrt{M}  + d^{-1} T^{\frac{1}{3}} M   } \ . 
\end{eqnarray*}
The last inequality follows from Cauchy $ \sum_{c \in F} \sqrt{p_c} \leq \sum_{c=1}^{M} \sqrt{p_c} \leq \sqrt{ \sum_{j=1}^{M} p_c  } = \sqrt{M}$. 
% Therefore, for contexts in $F$ we can control the estimation error to $2 \varepsilon_{(c)}$ and for contexts in $F^\complement$, we will not meet them very often, and hence the bound \Renyuan{explain mathematically how to get the first inequality.}

\item For the second term in \eqref{eq:upper_bound_three_terms_context}, 
let $\bar{A}^c $ be the random index of action taken in the exploitation phase when the context is $c$. 
Then, similar to the reasoning in \eqref{eq:thm_instance_independent_2}, it follows that  
\begin{eqnarray}
& & \E{ \sum_{t=1}^{T-1} \frac{1}{ (t+1)}  \sum_{s=1}^{t}  \left( \inner{\theta_*, A_{t+1}^{} - A_{s}^{} } \right)^2 }  \nonumber \\ 
&\leq& 4 n +  4 \E{  \sum_{t=n+1}^{T-1}  \frac{1}{ (t+1)}  \sum_{c=1}^{M}  \sum_{i=1}^{K} \one{Z_t=c} \one{ \bar{A}^c = i }  \sum_{i'=1}^{K} \sum_{c'=1}^{M}  \tau^{\operatorname{exp}}_{i', c'}   }   \nonumber \\ 
&=& 4 n +   4 \E{  \sum_{t=n+1}^{T-1}  \frac{1}{ (t+1)}  \sum_{c=1}^{M}  \sum_{i=1}^{K} \one{Z_t=c} \one{ \bar{A}^c = i } n   }  \nonumber \\ 
&=& 4 n +  4 \E{  \sum_{t=n+1}^{T-1}  \frac{1}{ (t+1)} n   }  \leq 4 n +  4 n \log\paren{T}  \ . 
\end{eqnarray}
Here, in the first inequality we used the fact that length of the exploration phase is $n$ and $\Gamma_{i,j} \leq 4$.  
The first equation follows simply because length of the exploration phase is $n$ and hence $\sum_{i'=1}^{K} \sum_{c'=1}^{M}  \tau^{\operatorname{exp}}_{i', c'} = n $.
The second equation holds since there can be only action taken at any time point. 
\end{enumerate}
Now the proof is complete.
