# Supplementary material for: Risk-Aware Linear Bandits: Theory and Applications in Smart Order Routing
Source: arXiv:2208.02389 source file (2026-04-02)
Supplement: Supplementary file 2 [file appendix_nonstationary_original.tex]

\section{A Non-Stationary Setting}
In this section, we consider a piecewise stationary setting similar to \cite{garivier2008upper, yu2009piecewise, auer2008near}, to showcase that our analysis can be potentially extended to more challenging settings than the stationary setting. 

For simplicity, we assume that the variances of different arms are the same. 
We note that it is possible to extend the analysis to a more general setting where the variances of different actions are not identical, following the approach outlined in the main body.
In what follows, we assume that the reward at time $t$ is generated by 
\begin{equation}
    X_t = \inner{\theta_t, A_t} + \eta_t ,~~\eta_t \sim \mathcal{N}(0, \sigma^2)  \ ,
\end{equation}
where $\eta_t$'s are sampled in an i.i.d. fashion. 
We assume that $\normtwo{A_t} \leq L_a, \normtwo{\theta_t} \leq L_{\theta}$. 
The coefficient $\theta_t$ is allowed to change (abruptly) $\Upsilon_T$ many times throughout the horizon of $T$ steps. 
We assume that we have the knowledge of $T$ and $\Upsilon_T$ in advance. \Jingwei{@ Ruihao: Can we claim that it is possible to extend to the case where $\Upsilon_T$ is unknown in advance? }
We define the variation of coefficients over $T$ steps to be $\mathcal{V}_T = \sum_{t=1}^{T} \normtwo{ \theta_t - \bar{\theta}_T }^2 $, where $\bar{\theta}_T = \frac{1}{T} \sum_{t=1}^{T} \theta_t $.
Given a policy $\pi$, the expected MV is again 
\begin{eqnarray}
    & & \E{ \sum_{t=1}^T\left(X_t^\pi-\frac{1}{T}\sum_{s=1}^T X_{s}^\pi \right)^2 - \rho \sum_{t=1}^{T} X^{\pi}_{t}}   \ .  \nonumber 
\end{eqnarray}
Our benchmark is the best single-arm policy. 

The overall idea of our strategy is simple. Given this piecewise stationary setting where $\theta_t$'s are assumed to change abruptly, we will restart our algorithm \rise~ every $H$ steps to adapt to this non-stationarity. 
We evenly divide $T$ rounds to $P = \lceil \frac{T}{H} \rceil$ periods.
Let $\tau_h$ be the length of period $h$. 
Because of the rounding issue, we set the lengths of the first $P-1$ periods to be $ H $. 
Hence, the length of the last period is $T - ( \lceil \frac{T}{H} \rceil -1) H \leq H $. 
Within each period, we deploy one instance of \rise~algorithm, with parameter $\varepsilon_h = \tilde{\Theta} \paren{  d H^{- \frac{1}{2}} }$ and $\delta_h = \frac{1}{H}$.  
Hence, each period consists of a complete exploration-and-exploitation cycle. 
This way, there are two sources of regret: 
\begin{itemize}
    \item For periods without any changes, leveraging the results from the stationary setting, the regret incurred during such a period can be upper bounded by $ \tilde{O}(H^{\frac{2}{3}}) $. 
    Since there are a total of $ \Theta(\frac{T}{H}) $ periods, the cumulative regret from this part is bounded by $ \tilde{O}(H^{\frac{2}{3}} \cdot \frac{T}{H}) = \tilde{O} \paren{ H^{ - \frac{1}{3} } T  } $. 
    \item The total regret from each period when there is indeed a change is at most $O(H)$. Since there are $\Upsilon_T$ changes, the cumulative regret due to changing periods is upper bounded by $O \paren{H \Upsilon_T}$. 
\end{itemize}

However, as observed in the stationary setting, the quantity MV is not immediately decomposable in time. 
To proceed with the previous argument, we require an appropriate decomposition of the accumulated MV regret, as stated below. 
\begin{lemma}
Let $X_t^a$ be the reward obtained at time $t$ by selecting action $a$. 
For any $a \in \mathcal{A}$, the expected MV regret incurred by a policy $\pi$ compared to a single arm policy is upper bounded by 
    \begin{eqnarray}
         & & \E{ \sum_{t=1}^T\left(X_t^\pi-\frac{1}{T}\sum_{s=1}^T X_{s}^\pi \right)^2 - \rho \sum_{t=1}^{T} X^{\pi}_{t}}  
         - \E{ \sum_{t=1}^T\left(X_t^a-\frac{1}{T}\sum_{s=1}^T X_{s}^a \right)^2 - \rho \sum_{t=1}^{T} X^{a}_{t}}  \nonumber \\ 
         &\lesssim&  L_a^2 \mathcal{V}_T 
         + \sum_{t=1}^{T-1}  \E{ \frac{1}{t+1} \sum_{s=1}^{t} \paren{ \inner{ \theta_s, A_{t+1}-A_{s} } }^2  } 
         + \rho \E{ \sum_{t=1}^{T} \inner{\theta_t , a - A_t } }  
         + \sigma L_a L_{\theta}  \sqrt{T}   \ . 
    \end{eqnarray}
\end{lemma}

Let $a^*$ be the best single arm in hindsight.

% Let the length of each period be $\lfloor \frac{T}{H} \rfloor$
$$
G_h = \braces{  \abs{} \leq \varepsilon_h, ~~ \forall~ a \in \mathcal{A} }  
$$

For ease of exhibition, we introduce some notations for time index. 
Let $s_h$ denote the time index at which the exploration phase ends in period $h$.
Similarly, let $e_h$ denote the time index at which the exploitation phase ends in period $h$.
Let $e_0 = 0$. 

\begin{eqnarray}
    & &  \E{ \sum_{t=1}^{T} \inner{\theta_t , a - A_t } } =   \sum_{h=1}^{P} \E{  \sum_{t=e_{h-1}+1}^{s_h }   \inner{\theta_t , a - A_t } 
    +  \sum_{t=s_h+1 }^{ e_h }   \inner{\theta_t , a - A_t } }     \nonumber \\ 
    &\leq&    \sum_{h=1}^{P}  \paren{ 2 L_a L_{\theta} n_h 
    +  \E{  \sum_{t=s_h+1 }^{ e_h }   \inner{\theta_t , a - A_t } } }  \nonumber \\ 
    &\lesssim& L_a L_\theta \lceil \frac{T}{H} \rceil d H^{\frac{2}{3}} +   \sum_{h=1}^{P}  \E{  \sum_{t=s_h+1 }^{ e_h }   \inner{\theta_t , a - A_t } }   
\end{eqnarray}

\begin{eqnarray}
 & & \sum_{h=1}^{P}  \sum_{t=s_h+1}^{ e_h } \E{ \inner{ \theta_t , a^* - A_t } }  \nonumber \\ 
 &\leq&  \sum_{h=1}^{P}  \sum_{t=s_h+1}^{ e_h } 
 \paren{ \E{ \inner{ \theta_t - \hat{\theta}_t , a^*  } 
 + \inner{ \hat{\theta}_t, a^* - A_t } 
 + \inner{ \hat{\theta}_t - \theta_t , A_t  } 
 ~\Big |~ G_h } \p{ G_h }
 + 2 L_a L_\theta \p{ G_{h}^{\complement} } } \nonumber \\ 
 &\leq&  \sum_{h=1}^{P}  \sum_{t=s_h+1}^{ e_h } 
 \paren{ \E{ \abs{  \inner{ \theta_t - \hat{\theta}_t , a^*  } } 
 + \abs{ \inner{ \hat{\theta}_t - \theta_t , A_t  } } 
 ~\Big |~ G_h } \p{ G_h }
 + 2 L_a L_\theta \p{ G_{h}^{\complement} } } \nonumber  \\ 
 &\leq& \sum_{h=1}^{P}  \sum_{t=s_h+1}^{ e_h } 
 \paren{ 2 \varepsilon_h 
 + 2 L_a L_\theta \delta_h  }  \nonumber   \\ 
 &\lesssim&  \sum_{h=1}^{P} \paren{ H - n_h } \paren{ d H^{ - \frac{1}{3} } + L_a L_\theta \frac{1}{H} }   \nonumber \\
 &\lesssim& \lceil \frac{T}{H} \rceil d H^{\frac{2}{3}} \ . 
\end{eqnarray}

\Jingwei{There is a fatal mistake below: Need to fix. }

% $\mathcal{T}_1, \cdots, \mathcal{T}_H$

\begin{eqnarray}
    & & \sum_{t=1}^{T-1}   \frac{1}{t+1} \sum_{s=1}^{t} \E{ \paren{ \inner{ \theta_s, A_{t+1}-A_{s} } }^2  } 
     \nonumber \\  %  \sum_{t \in \mathcal{T}_h} 
    &\lesssim& \sum_{h=1}^{P} \brackets{ n_h \Gamma_{\max}^2 + \sum_{t = s_h}^{ e_h } \frac{1}{t+1} \sum_{s=1}^{t} \E{ \paren{ \inner{ \theta_s, A_{t+1}-A_{s} } }^2  }       }   \\
    &=&  \sum_{h=1}^{P} \brackets{ n_h \Gamma_{\max}^2 + \sum_{t = s_h + 1 }^{ e_h } \frac{1}{t+1} \sum_{s=1}^{s_h} \E{ \paren{ \inner{ \theta_s, A_{t+1}-A_{s} } }^2  }       }
\end{eqnarray}

Within the period when there is no change, we will re-use the result in to conclude that

\begin{myproof}

Following the same reasoning as \eqref{eq:per_round_regret_decomposition_1}, we have 
$$
 \E{  \sum_{t=1}^T\left(X_t-\frac{1}{T}\sum_{s=1}^T X_{s} \right)^2  } =  \sum_{t=1}^{T-1} \E{  \frac{1}{t(t+1)} \paren{ t X_{t+1} - \sum_{s=1}^{t} X_s }^2 }  \ . 
$$
We can further decompose the summand in the following way: 
\begin{eqnarray}
    & & \E{ \frac{1}{t(t+1)} \paren{ t X_{t+1} - \sum_{s=1}^{t} X_s }^2 } \nonumber  \\
    &=& \E{  \frac{1}{t(t+1)} \paren{ t \inner{\theta_{t+1}, A_{t+1}} + t \eta_{t+1} - \sum_{s=1}^{t} ( \inner{\theta_s, A_s} + \eta_s )  }^2   }  \nonumber \\
    &=& \E{  \frac{1}{t(t+1)} \paren{ t \inner{\theta_{t+1}, A_{t+1}} -  \sum_{s=1}^{t} \inner{\theta_s, A_s} }^2 }  \label{eq:nonstationary_summand_1} \\
    & & + \E{ \frac{1}{t(t+1)}  \paren{ t \eta_{t+1} - \sum_{s=1}^{t} \eta_s   }^2 }  \label{eq:nonstationary_summand_2} \\ 
    & & + \E{  \frac{2}{t(t+1)}  \paren{t \inner{\theta_{t+1}, A_{t+1}} -  \sum_{s=1}^{t} \inner{\theta_s, A_s}  } \paren{  t \eta_{t+1} - \sum_{s=1}^{t} \eta_s  } }  \label{eq:nonstationary_summand_3} \ . 
\end{eqnarray}

Next, we analyze these three terms respectively. 
\begin{itemize}[left=1cm]
    \item  Regarding the term \eqref{eq:nonstationary_summand_1}, we notice that 
    \begin{eqnarray}
    & & \E{  \frac{1}{t(t+1)} \paren{ t \inner{\theta_{t+1}, A_{t+1}} -  \sum_{s=1}^{t} \inner{\theta_s, A_s} }^2 }  \nonumber \\
    &=& \E{  \frac{1}{t(t+1)}  \paren{
    \inner{ \sum_{s=1}^{t} \paren{ \theta_{t+1} - \theta_s }, A_{t+1} }
   + \sum_{s=1}^{t}  \inner{ \theta_s, A_{t+1} - A_s }  }^2}  \nonumber \\
   &\lesssim& \E{ \frac{1}{t(t+1)}  \paren{
    \inner{ t \theta_{t+1} - \sum_{s=1}^{t} \theta_s , A_{t+1} } }^2
   + \frac{1}{t(t+1)} \paren{ \sum_{s=1}^{t}  \inner{ \theta_s, A_{t+1} - A_s }  }^2   }   \\ 
   &\leq& \E{ \frac{1}{t(t+1)}  
    \normtwo{t \theta_{t+1} - \sum_{s=1}^{t} \theta_s }^2 \normtwo{A_{t+1}}^2
   + \frac{1}{t(t+1)} \paren{ \sum_{s=1}^{t}  \inner{ \theta_s, A_{t+1} - A_s }  }^2   }  \\
   &\leq& L_a^2 \frac{1}{t(t+1)}  \normtwo{t \theta_{t+1} - \sum_{s=1}^{t} \theta_s }^2
   +  \E{  \frac{1}{t+1} \sum_{s=1}^{t} \paren{ \inner{ \theta_s, A_{t+1}-A_{s} } }^2 }  \ . 
\end{eqnarray}
Therefore, if we sum over $t$, in view of Lemma~\ref{lemma:sum_variation} (stated at the end of this section) we get 
\begin{eqnarray}
    & & \sum_{t=1}^{T-1} \E{  \frac{1}{t(t+1)} \paren{ t \inner{\theta_{t+1}, A_{t+1}} -  \sum_{s=1}^{t} \inner{\theta_s, A_s} }^2 }   \nonumber \\  
    &\lesssim&  L_a^2 \mathcal{V}_T + \sum_{t=1}^{T-1}  \E{  \frac{1}{t+1} \sum_{s=1}^{t} \paren{ \inner{ \theta_s, A_{t+1}-A_{s} } }^2 }   \ . 
\end{eqnarray}
    \item The term \eqref{eq:nonstationary_summand_2} is easy to control: 
    \begin{equation}
         \E{  \paren{ t \eta_{t+1} - \sum_{s=1}^{t} \eta_s   }^2 } 
    =  \sum_{i=1}^{t} \sum_{j=1}^{t} \E{ \eta_{t+1}^2 - \eta_{t+1} \eta_i - \eta_{t+1} \eta_j + \eta_i \eta_j  }   
    = t^2 \E{ \eta_{t+1}^2} + \sum_{s=1}^{t} \E{ \eta_{s}^{2} }  
    = (t^2+t) \cdot \sigma^2  \nonumber   \ . 
    \end{equation}
    \item  The term \eqref{eq:nonstationary_summand_3} contributes to the square root term in the bound 
    \begin{eqnarray} 
        & &  \E{  \frac{2}{t(t+1)}  \paren{t \inner{\theta_{t+1}, A_{t+1}} -  \sum_{s=1}^{t} \inner{\theta_s, A_s}  } \paren{  t \eta_{t+1} - \sum_{s=1}^{t} \eta_s  } }   \nonumber  \\ 
        &=& \frac{2}{t(t+1)} \E{ \paren{t \inner{\theta_{t+1}, A_{t+1}} -  \sum_{s=1}^{t} \inner{\theta_s, A_s}  } t \eta_{t+1} }
     - \frac{2}{t(t+1)} \E{  \paren{t \inner{\theta_{t+1}, A_{t+1}} -  \sum_{s=1}^{t} \inner{\theta_s, A_s}  } \sum_{s=1}^{t} \eta_s }  \nonumber \\ 
     &=& \frac{2}{t(t+1)} \E{  \paren{t \inner{\theta_{t+1}, A_{t+1}} -  \sum_{s=1}^{t} \inner{\theta_s, A_s}  } \sum_{s=1}^{t} \eta_s }   \label{eq:nonstationary_noise_ignore}  \\ 
     &\lesssim& \sigma_{} L_a L_{\theta} \frac{1}{ \sqrt{t} }  \nonumber \ ,  
    \end{eqnarray}
\Jingwei{Something does not feel right here... You need to take into account that $\theta$ is changing!!! }
where \eqref{eq:nonstationary_noise_ignore} follows from the same reasoning as \eqref{eq:noise_term_can_ignore}, and the final step is justified using the same argument as \eqref{eq:noise_term_3}.
\end{itemize}

Now, it remains to lower bound $ \E{ \sum_{t=1}^T\left(X_t^a-\frac{1}{T}\sum_{s=1}^T X_{s}^a \right)^2 - \rho \sum_{t=1}^{T} X^{a}_{t}} $. 
To this end, we observe that 
\begin{eqnarray}
    &  &   \E{ \sum_{t=1}^T\left(X_t^a-\frac{1}{T}\sum_{s=1}^T X_{s}^a \right)^2 }  \nonumber  \\ 
    &=&  \E{ \sum_{t=1}^{T} (X_t^a)^2 - T (\bar{X}_T^a)^2 }  
    =  \sum_{t=1}^{T} \E{ (X_t^a)^2 }  - \frac{1}{T} \E{ \sum_{t=1}^{T} X_t^a  \sum_{s=1}^{T} X_s^a  }  \nonumber \\
    &=&  \sum_{t=1}^{T}  \paren{ \sigma^2 + \inner{\theta_t, a}^2  }    - \frac{1}{T} \brackets{ \sum_{t=1}^{T} \paren{ \sigma^2 + \inner{\theta_t, a}^2  }  + \sum_{s \neq t}^{T}  \inner{\theta_t, a} \inner{\theta_s, a}  } \nonumber  \\
    &=& (T-1) \sigma^2 + \sum_{t=1}^{T} \inner{\theta_t, a}^2   - \frac{1}{T} \sum_{t=1}^{T} \sum_{s=1}^{T} \inner{\theta_t, a} \inner{\theta_s, a}  \nonumber   \\
    &\geq& (T-1) \sigma^2  \ ,  \nonumber
\end{eqnarray}
where the last step follows from Cauchy's inequality.

\begin{lemma} \label{lemma:sum_variation}
\begin{equation}
    \sum_{k=1}^{n+1} \normtwo{ \theta_k - \bar{\theta}_{n+1} }^2   =  \sum_{k=1}^{n} \normtwo{ \theta_k - \bar{\theta}_{n} }^2   +  \frac{1}{n(n+1)} \normtwo{ n \theta_{n+1} - n  \bar{\theta}_n  }^2  
\end{equation}
\end{lemma}
The proof follows from straightforward calculation. 
We include it here only for completeness. 
We first note that 
\begin{eqnarray*}
     \sum_{k=1}^{n+1} \normtwo{ \theta_k - \bar{\theta}_{n+1} }^2 &=& \normtwo{\theta_{n+1} - \bar{\theta}_{n+1}}^2 
     +  \sum_{k=1}^{n} \normtwo{ \theta_k - \bar{\theta}_{n} + \bar{\theta}_{n} - \bar{\theta}_{n+1} }^2  \\ 
     &=& \normtwo{\theta_{n+1} - \bar{\theta}_{n+1}}^2 
     +  \sum_{k=1}^{n}   \paren{  \normtwo{ \theta_k - \bar{\theta}_n   }^2 
     + \normtwo{ \bar{\theta}_{n} - \bar{\theta}_{n+1} }^2  
     + 2 \inner{ \theta_k - \bar{\theta}_{n} ,  \bar{\theta}_{n} - \bar{\theta}_{n+1} }   }    \\ 
     &=& \normtwo{\theta_{n+1} - \bar{\theta}_{n+1}}^2 
     +  \sum_{k=1}^{n}   \normtwo{ \theta_k - \bar{\theta}_n   }^2 + n \normtwo{ \bar{\theta}_{n} - \bar{\theta}_{n+1} }^2 
     + 2 \inner{ \sum_{k=1}^{n} ( \theta_k - \bar{\theta}_{n}) ,  \bar{\theta}_{n} - \bar{\theta}_{n+1} }  \\ 
     &=&  \normtwo{\theta_{n+1} - \bar{\theta}_{n+1}}^2 
     + n \normtwo{ \bar{\theta}_{n} - \bar{\theta}_{n+1} }^2
     + \sum_{k=1}^{n}   \normtwo{ \theta_k - \bar{\theta}_n   }^2  \\
     &=&  \sum_{k=1}^{n} \normtwo{ \theta_k - \bar{\theta}_{n} }^2   +  \frac{1}{n(n+1)} \normtwo{ n \theta_{n+1} - n  \bar{\theta}_n  }^2  \ ,
\end{eqnarray*}
where the last step follows from the fact that 
\begin{eqnarray*}
    & &  \normtwo{\theta_{n+1} - \bar{\theta}_{n+1}}^2  + n \normtwo{ \bar{\theta}_{n} - \bar{\theta}_{n+1} }^2 \\ 
    &=&  \normtwo{\theta_{n+1} -  \frac{1}{n+1} \paren{ \theta_{n+1} + n \bar{\theta}_{n} }  }^2  
    + n \normtwo{ \frac{ \sum_{k=1}^{n} \theta_k  }{n}  - \frac{ \theta_{n+1} + \sum_{k=1}^{n} \theta_k }{n+1} }^2  \\ 
    &=&   \normtwo{ \frac{1}{n+1} \paren{ n \theta_{n+1} - n \bar{\theta}_n }  }^2  
    + n \normtwo{ \frac{1}{(n+1)n} \paren{ \theta_{n+1} + n \bar{\theta}_{n} }   }^2  \\
    &=& \frac{1}{(n+1)n} \normtwo{ n \theta_{n+1} - n \bar{\theta}_n }^2  \ . 
\end{eqnarray*}
\end{myproof}
