# Supplementary material for: Risk-Aware Linear Bandits: Theory and Applications in Smart Order Routing
Source: arXiv:2208.02389 source file (2026-04-02)
Supplement: Supplementary file 3 [file appendix.tex]

\begin{APPENDIX}{Omitted Proofs}

\section{Proof of Proposition \ref{prop:bound_ip}}\label{sec:prop:bound_ip}

From Eq. (21.1) of \cite{lattimore2020bandit}), we have for any fixed $n,$ $\delta > 0$, and every $a\in\cA,$
\begin{align} \label{eq:bound_inner_product_theta}
    \p{ \left|\langle\hat{\theta}_{n} - \theta_{*},a \rangle\right|  \geq  \sigma_{\max} \sqrt{2\|a\|^2_{V^{-1}_n}\log \left( 2\delta^{-1} \right)} } \leq \delta.
\end{align}
Then from theorem 1 of \cite{stay2019},
we have for any fixed $n,$ $\delta > 0$, and every $a\in\cA,$
\begin{equation}
\left | \innerprdct{ \hat{\phi}_{n} - \phi_{*}, a}  \right | \leq C_3\left \|a \right \|_{V_{n}^{-1}} d\sqrt{\log(d)}\log(2\delta^{-1}). \label{eq:bound_inner_product_phi}
\end{equation}
By a union bound over \eqref{eq:bound_inner_product_theta} and \eqref{eq:bound_inner_product_phi}, we have for any fixed $n,$ $\delta>0$, and every $a\in\cA,$ it holds with probability at least $1 - \delta$, that
\begin{align}
 & \left | \innerprdct{a, \phi_{*} - \rho \theta_{*}} - \innerprdct{a, \hat{\phi}_{n} - \rho \hat{\theta}_{n}  } \right | \nonumber \\
\leq&  \rho \left | \innerprdct{a, \theta_{*} - \hat{\theta}_{n} } \right | + \left | \innerprdct{a, \phi_{*} - \hat{\phi}_{n} }\right |       \nonumber \\ 
\leq& \left \| a \right \|_{V_{n}^{-1}} \rho \sigma_{\max} \sqrt{2 \log \left(4\delta^{-1}\right)}  +  
C_3\left \|a \right \|_{V_{n}^{-1}} d\sqrt{\log(d)}\log(4\delta^{-1}) \nonumber \\
\leq&  \left \|a \right \|_{V_{n}^{-1}} \tilde{C} d \sqrt{  \log{(d)} }  \log( {\delta^{-1}}), \label{eq:bound_ip}
\end{align}
where the second step follows from triangle inequality and the last step follows from the definition of $\tilde{C}.$

Now recall the definition of $n_a$ in \eqref{eq:n_a}, we have
\begin{align}
V_n =& \sum_{a \in \mathcal{A}} n_a a a^\top  = \sum_{a \in \mathcal{A}} \left \lceil  \frac{ \tilde{C}^2 \log^2 \left( \delta^{-1}\right) d^2 \log{(d)} g(Q^*) Q^* (a)  }{\varepsilon^2}   \right \rceil a a^\top \nonumber  \\
\succeq& \sum_{a \in \mathcal{A}} \frac{ \tilde{C}^2 \log^2 \left( \delta^{-1}\right) d^2 \log{(d)} g(Q^*) Q^* (a)   }{\varepsilon^2}  a a^{\top} \nonumber \\ 
=& \frac{ \tilde{C}^2 \log^2 \left( \delta^{-1}\right) d^2 \log{(d)} g(Q^*)}{\varepsilon^2}\sum_{a\in\cA}Q^*(a)aa^{\top},
\end{align}
where we denote by $B \succeq 0$ if the matrix $B$ is positive semi-definite. Hence, we arrive at
\begin{align}
\left \|a \right \|_{V_{n}^{-1}}  =& \sqrt{ a^\top V_{n}^{-1} a }  \nonumber \leq \sqrt{ \frac{\varepsilon^2a^\top (\sum_{a\in\cA}Q^*(a)aa^{\top})^{-1} a}{ \tilde{C}^2 \log^2 \left( \delta^{-1}\right) d^2 \log( d)  g(Q^*)} }  \nonumber \\
\leq& \frac{\varepsilon}{ \tilde{C} d \sqrt{\log(d)}\log \left(\delta^{-1}\right)    }   ,  \label{eq:a_norm}
\end{align}
where the last step follows from the fact that $Q^*$ is an optimal solution to \eqref{eq:g-optimal}. The statement follows by combining \eqref{eq:bound_ip} and \eqref{eq:a_norm}.

\iffalse
Denote by $D_{\tau} = \left[A_1 ~~A_2~~ \cdots ~~A_{\tau} \right]^{\top}$.  
To proceed, we first investigate the expression of $\hat{\phi}_{\tau} $. 
\begin{eqnarray*}
 \hat{\phi}_{\tau} &=& ( D_{\tau}^{\top} D_{\tau} )^{-1} D_{\tau}^{\top} f^{-1} ( \hat{\eta}_{\tau} \circ \hat{\eta}_{\tau} ) \\
 &=& ( D_{\tau}^{\top} D_{\tau} )^{-1} D_{\tau}^{\top}  \left ( f^{-1} ( \hat{\eta}_{\tau} \circ \hat{\eta}_{\tau} ) - D_{\tau} \phi_{*}  \right )  + \phi_{*} .
\end{eqnarray*}
Hence, for any $x \in \mathbb{R}^{d}$, 
\begin{eqnarray*}
& & \mid \innerprdct{ x , \hat{\phi}_{\tau} - \phi_{*} }  \mid \\ 
&=& \mid x^{\top}  ( D_{\tau}^{\top} D_{\tau} )^{-1} D_{\tau}^{\top}  \left ( f^{-1} ( \hat{\eta}_{\tau} \circ \hat{\eta}_{\tau} ) - D_{\tau} \phi_{*}  \right )  \mid \\
 &\leq& \left \| x^{\top}  ( D_{\tau}^{\top} D_{\tau} )^{-1} \right \|_{V_{\tau}} \cdot  \left \| D_{\tau}^{\top}  \left ( f^{-1} ( \hat{\eta}_{\tau} \circ \hat{\eta}_{\tau} ) - D_{\tau} \phi_{*}  \right ) \right \|_{V_{\tau}^{-1}}  \\
 &=&  \left \|x  \right  \|_{V_{\tau}^{-1}}  \cdot  \left \| D_{\tau}^{\top}  \left ( f^{-1} ( \hat{\eta}_{\tau} \circ \hat{\eta}_{\tau} ) - D_{\tau} \phi_{*}  \right ) \right \|_{V_{\tau}^{-1}}  \\
 &=& \left \|x \right \|_{V_{\tau}^{-1}}  \cdot \left \| D_{\tau}^{\top}  \left ( f^{-1} ( (\hat{\eta}_{\tau} - \eta_{\tau} + \eta_{\tau}) \circ (\hat{\eta}_{\tau} - \eta_{\tau} + \eta_{\tau}) ) - D_{\tau} \phi_{*}  \right ) \right \|_{V_{\tau}^{-1}}  \\
 &\leq&  \left \|x \right \|_{V_{\tau}^{-1}} \cdot \Big( \left \| D_{\tau}^{\top}  \left ( f^{-1} (\eta_{\tau} \circ \eta_{\tau} ) - D_{\tau} \phi_{*}  \right ) \right \|_{V_{\tau}^{-1}} \\
 & & +   2 \left \|  D_{\tau}^{\top} \left( \eta_{\tau} \circ D_{\tau}\left(\theta_{*}-\hat{\theta}_{\tau}\right)  \right) \right \|_{V_{\tau}^{-1}}  \\ 
 & & 
 +  \left \| D_{\tau}^{\top} \left( D_{\tau} \left(\theta_{*}-\hat{\theta}_{\tau}\right)  \circ \left(\theta_{*}-\hat{\theta}_{\tau}\right)   \right) \right \|_{V_{\tau}^{-1}}    \Big) . 
\end{eqnarray*}

Now we resort to several results from \cite{stay2019} which we restate in the following lemma. 
\begin{lemma} 
[Results from \cite{stay2019}] \label{lemma:restate}
\begin{enumerate}
\item For any $\tau \in \mathbb{N}$, for any $\delta > 0$, with probability at least $1 - \delta$, we have 
    \begin{equation}
    \left \| D_{\tau}^{\top}  \left ( f^{-1} (\eta_{\tau} \circ \eta_{\tau} ) - D_{\tau} \phi_{*}  \right ) \right \|_{V_{\tau}^{-1}} \leq \alpha^{(2)}(\delta).    
    \end{equation}
    
\item Let $H_{\tau} = \operatorname{Diag}(\eta_1, \eta_2, \cdots, \eta_{\tau})$. We have 
    \begin{equation}
    \left \|  D_{\tau}^{\top} \left( \eta_{\tau} \circ D_{\tau}\left(\theta_{*}-\hat{\theta}_{\tau}\right)  \right)  \right \|_{V_{\tau}^{-1}} \leq \left \| V_{\tau}^{-\frac{1}{2}} D_{\tau}^{\top} H_{\tau} D_{\tau}^{} V_{\tau}^{-\frac{1}{2}}   \right \|_{2} \cdot
    \left \| \theta_{*}-\hat{\theta}_{\tau} \right \|_{V_{\tau}} . 
    \end{equation}
    Moreover, for any $\tau \in \mathbb{N}$, for any $\delta > 0$, we have 
    \begin{equation}
    \p{  \left \| V_{\tau}^{-\frac{1}{2}} D_{\tau}^{\top} H_{\tau} D_{\tau}^{} V_{\tau}^{-\frac{1}{2}}  \right \|_2 \geq \alpha^{(3)}(\delta) } \leq \delta.  
    \end{equation}

\item For any $\tau \in \mathbb{N}$,
    \begin{equation}
     \left \| D_{\tau}^{\top} \left( D_{\tau} \left(\theta_{*}-\hat{\theta}_{\tau}\right)  \circ \left(\theta_{*}-\hat{\theta}_{\tau}\right)   \right) \right \|_{V_{\tau}^{-1}} \leq  \left \| \theta_{*}-\hat{\theta}_{\tau} \right \|_{V_{\tau}}^{2}    .
    \end{equation}
\end{enumerate}

\end{lemma}
\paragraph{Remark.} Part 1 is from Lemma 3 of \cite{stay2019}. Part 2 follows from Eq. 94 and Eq. 106. Part 3 is a direct consequence of Eq. 120. 

Regarding the OLS estimator for $\theta_*$, we know for given $\tau \in \mathbb{N}$ and $\delta > 0 $,
$$
\p{ \| \hat{\theta}_{\tau} - \theta_{*} \|_{V_{\tau}}  \geq 4 \sqrt{2} \sigma_{\max} \sqrt{d + \log \left( \frac{1}{\delta} \right)} } \leq \delta.
$$

Combining it with Lemma~\ref{lemma:restate} together yields that, for any $x \in \mathbb{R}^d$, with probability at least $1- \delta$, 
\begin{eqnarray}
 &&\mid \innerprdct{ x , \hat{\phi}_{\tau} - \phi_{*} }  \mid \\
 &\leq&  \left \|x \right \|_{V_{\tau}^{-1}} \cdot \Big (  \left \| D_{\tau}^{\top}  \left ( f^{-1} (\eta_{\tau} \circ \eta_{\tau} ) - D_{\tau} \phi_{*}  \right ) \right \|_{V_{\tau}^{-1}}  \nonumber \\ 
 & & + 2 \left \| V_{\tau}^{-\frac{1}{2}} D_{\tau}^{\top} H_{\tau} D_{\tau}^{} V_{\tau}^{-\frac{1}{2}}   \right \|_{2} \left \| \theta_{*}-\hat{\theta}_{\tau} \right \|_{V_{\tau}}  + \left \| \theta_{*}-\hat{\theta}_{\tau} \right \|_{V_{\tau}}^{2}  \Big )   \nonumber  \\
 &\leq&  \left \|x \right \|_{V_{\tau}^{-1}} \cdot \left ( \alpha^{(2)}(\frac{\delta}{3}) + 2 \alpha^{(3)}(\frac{\delta}{3}) \alpha^{(4)}(\frac{\delta}{3}) + \alpha^{(4)}(\frac{\delta}{3})^2 \right) \nonumber \\
 &=& \left \|x \right \|_{V_{\tau}^{-1}} \cdot  \zeta(\delta) . \label{eq:bound_inner_product_phi}  
\end{eqnarray}
\Jingwei{Finish this..}
In view of Eq.~\eqref{eq:bound_inner_product_theta} and Eq.~\eqref{eq:bound_inner_product_phi}, with probability at least $1 - \delta$, we have 
\begin{eqnarray}
& & \left | \innerprdct{a, \phi_{*} - \rho \theta_{*}} - \innerprdct{a, \hat{\phi}_{\tau} - \rho \hat{\theta}_{\tau}  } \right | \nonumber \\
&\leq&  \rho \left | \innerprdct{a, \theta_{*} - \hat{\theta}_{\tau} } \right | + \left | \innerprdct{a, \phi_{*} - \hat{\phi}_{\tau} }\right |       \nonumber \\ 
&\leq& \left \| a \right \|^{}_{V_{\tau}^{-1}} \cdot \rho \sigma_{\max} \sqrt{2 \log \left( \frac{4}{\delta}\right)}  +  
\left \|a \right \|_{V_{\tau}^{-1}} \cdot \zeta(\frac{\delta}{2}) \nonumber \\
&\leq&  \left \|a \right \|_{V_{\tau}^{-1}} \cdot \tilde{C} d \sqrt{  \log{(d)} }  \log \left( {\frac{1}{\delta}} \right)  . \label{eq:bound_inner_product_MV_1}
\end{eqnarray}
\fi 


\section{Proof of Proposition \ref{prop:regret_trans}} \label{sec:prop:regret_trans}
We first define the empirical mean of the algorithm over the entire time horizon $[T]$ as
\begin{align}\label{eq:inter0}
    \hat{\mu}=\frac{1}{T}\sum_{t=1}^TX_t=\frac{1}{T}\sum_{a\in\cA}\tau_a(T)\hat{\mu}_a,
\end{align}
where $\hat{\mu}_a=(\sum_{t=1}^TX_t\bm{1}[A_t=a])/\tau_a(T)$ is the empirical mean of action $a$ over $[T].$ Defining $\hat{\sigma}_a=(\sum_{t=1}^T(X_t-\hat{\mu}_a)^2\bm{1}[A_t=a])/\tau_a(T)$ as the empirical variance of action $a$ over $[T],$ the empirical variance of the algorithm over $[T]$ is thus
\begin{align}
    \nonumber&\hat{\sigma}^2\\
    \nonumber=&\frac{1}{T}\sum_{t=1}^T(X_t-\hat{\mu})^2\\
    \nonumber=&\frac{1}{T}\sum_{a\in\cA}\sum_{t=1}^T(X_t-\hat{\mu})^2\bm{1}[A_t=a]\\
    \nonumber=&\frac{1}{T}\sum_{a\in\cA}\sum_{t=1}^T(X_t-\hat{\mu}_a+\hat{\mu}_a-\hat{\mu})^2\bm{1}[A_t=a]\\
    \nonumber=&\frac{1}{T}\sum_{a\in\cA}\sum_{t=1}^T(X_t-\hat{\mu}_a)^2\bm{1}[A_t=a]+ \frac{1}{T}\sum_{a\in\cA}\sum_{t=1}^T(\hat{\mu}_a-\hat{\mu})^2\bm{1}[A_t=a]\\
    \nonumber&+\frac{1}{T}\sum_{a\in\cA}\sum_{t=1}^T2(X_t-\hat{\mu}_a)(\hat{\mu}_a-\hat{\mu})\bm{1}[A_t=a]\\
    \nonumber=&\frac{1}{T}\sum_{a\in\cA}\sum_{t=1}^T(X_t-\hat{\mu}_a)^2\bm{1}[A_t=a]+ \frac{1}{T}\sum_{a\in\cA}\sum_{t=1}^T(\hat{\mu}_a-\hat{\mu})^2\bm{1}[A_t=a]\\
    = &\frac{1}{T}\sum_{a\in\cA}\tau_a(T)\hat{\sigma}_a^2+\frac{1}{T}\sum_{a\in\cA}\tau_a(T)(\hat{\mu}_a-\hat{\mu})^2.\label{eq:inter1}
\end{align}
For the second term in \eqref{eq:inter1}, we have by \eqref{eq:inter0} that
\begin{align}
    \nonumber&\sum_{a\in\cA}\tau_a(T)(\hat{\mu}_a-\hat{\mu})^2\\
    \nonumber=&\sum_{a\in\cA}\tau_a(T)\left(\frac{1}{T}\sum_{b\in\cA}\tau_b(T)\hat{\mu}_a-\frac{1}{T}\sum_{b\in\cA}\tau_b(T)\hat{\mu}_b\right)^2\\
    \nonumber=&\sum_{a\in\cA}\tau_a(T)\left(\frac{1}{T}\sum_{b\in\cA}\tau_b(T)(\hat{\mu}_a-\hat{\mu}_b)\right)^2\\
    \nonumber\leq&\frac{T}{T^2}\sum_{a\in\cA}\tau_a(T)\left(\sum_{b\in\cA}\tau_b(T)(\hat{\mu}_a-\hat{\mu}_b)^2\right)\\
    =&\frac{1}{T}\sum_{a\in\cA}\sum_{b\in\cA,b\neq a}\tau_a(T)\tau_b(T)(\hat{\mu}_a-\hat{\mu}_b)^2,\label{eq:inter2}
\end{align}
where the second last step follows from the Cauchy-Schwarz inequality. Hence, we have from \eqref{eq:inter0} and \eqref{eq:inter1} that
\begin{align}
    \nonumber&\E{\hat{R}_{\pi}(T)}\\
    \nonumber=&\E{\xi_{\pi}(T)-\xi_{\hat{\pi}^*}(T)}\\
    \nonumber=&\E{\sum_{a\in\cA}\tau_a(T)(\hat{\sigma}_a^2-\rho\hat{\mu}_a)}-\E{\sum_{a\in\cA}\tau_a(T)(\sigma_{a_*}^2-\rho\mu_{a_*})}\\
    \nonumber&+\E{\sum_{a\in\cA}\tau_a(T)(\hat{\mu}_a-\hat{\mu})^2}\\
    \nonumber\leq&\E{\sum_{a\in\cA}\tau_a(T)(\hat{\sigma}_a^2-\rho\hat{\mu}_a)}-\E{\sum_{a\in\cA}\tau_a(T)(\sigma_{a_*}^2-\rho\mu_{a_*})}\\
   &+\frac{1}{T}\E{\sum_{a\in\cA}\sum_{b\in\cA,b\neq a}\tau_a(T)\tau_b(T)(\hat{\mu}_a-\hat{\mu}_b)^2}.\label{eq:inter3}
\end{align}
Here, the final step follows from \eqref{eq:inter2}. For the first two terms in \eqref{eq:inter3},
\begin{align}
    \nonumber&\E{\sum_{a\in\cA}\tau_a(T)(\hat{\sigma}_a^2-\rho\hat{\mu}_a)}-\E{\sum_{a\in\cA}\tau_a(T)(\sigma_{a_*}^2-\rho\mu_{a_*})}\\
    \nonumber=&\sum_{a\in\cA}\E{\tau_a(T)(\hat{\sigma}_a^2-\rho\hat{\mu}_a)\mid \tau_a(T)}-\E{\sum_{a\in\cA}\tau_a(T)(\sigma_{a_*}^2-\rho\mu_{a_*})}\\
    \nonumber=&\sum_{a\in\cA}\E{\E{\bm{1}[\tau_a(T)>0]\tau_a(T)(\frac{\tau_a(T)-1}{\tau_a(T)}\sigma^2_a-\rho\mu_a)\mid \tau_a(T)}}\\
    \nonumber&-\E{\sum_{a\in\cA}\tau_a(T)(\sigma_{a_*}^2-\rho\mu_{a_*})}\\
    \nonumber=&\sum_{a\in\cA}\E{\tau_a(T)(\sigma^2_a-\rho\mu_a-\sigma_{a_*}^2+\rho\mu_{a_*})}+\sum_{a\in\cA,Q^*(a)>0}\sigma^2_a\\
    \nonumber=&\sum_{a\in\cA}\E{\tau_a(T)}\Delta_a+\sum_{a\in\cA,Q^*(a)>0}\sigma^2_a\\
    \leq&\sum_{a\in\cA}\E{\tau_a(T)}\Delta_a+\frac{d(d+1)+2}{2}\sigma^2_{\max},\label{eq:inter4}
\end{align}
where the last step makes use of the fact that $Q^*$ has at most $d(d+1)/2$ non-zero entries and the \rise~algorithm would stick to a single action during the exploitation phase. For the last term of \eqref{eq:inter3},
\begin{align}
    \nonumber&\frac{1}{T}\E{\sum_{a\in\cA}\sum_{b\in\cA,b\neq a}\tau_a(T)\tau_b(T)(\hat{\mu}_a-\hat{\mu}_b)^2}\\
    \nonumber=&\frac{1}{T}\sum_{a\in\cA}\sum_{b\in\cA,b\neq a}\E{\E{\tau_a(T)\tau_b(T)(\hat{\mu}_a-\hat{\mu}_b)^2\mid \tau_a(T),\tau_b(T)}}\\
    \nonumber=&\frac{1}{T}\sum_{a\in\cA}\sum_{b\in\cA,b\neq a}\E{\tau_a(T)\tau_b(T)\Gamma^2_{a,b}}\\
    \nonumber&+\frac{1}{T}\sum_{a\in\cA}\sum_{b\in\cA,b\neq a}\E{\bm{1}[\tau_a(T),\tau_b(T)>0](\tau_a(T)\sigma^2_b+\tau_b(T)\sigma^2_{a})}\\
    \nonumber<&\frac{1}{T}\sum_{a\in\cA}\sum_{b\in\cA,b\neq a}\E{\tau_a(T)\tau_b(T)\Gamma^2_{a,b}}+(d(d+1)+2)\sigma^2_{\max},
\end{align}
where the last step follows the same argument as that of \eqref{eq:inter4}. Combining this and \eqref{eq:inter4}, we can conclude the statement.


\section{Proof of Proposition \ref{prop:eps}} \label{sec:prop:eps}
We define $\Delta_{\max}=(\sigma^2_{\max}-\sigma^2_{\min}+2\rho).$ For the first term of $\E{\tilde{R}_{\pi}(T)},$  since the exploration phase lasts for $n$ time periods and $\Delta_a\leq\Delta_{\max}$, by Proposition~\ref{prop:bound_ip}, we have with probability at least $1 - \delta$, 
\begin{align}
\sum_{a \in \mathcal{A}} \E{\tau_{a}(T)} \Delta_a  \leq n\Delta_{\max} + (T-n) \varepsilon.
\end{align}
For the second term of $\E{\tilde{R}_{\pi}(T)},$ since $\Gamma_{a,b}\leq 2$
\begin{align*}
 &\frac{1}{T} \sum_{a \in \mathcal{A}} \sum_{b \in \mathcal{A},b\neq a} \E{\tau_{a}(T)\tau_{b}(T)}  \Gamma_{a,b}^2 \\
 \leq&\frac{4}{T} \sum_{a \in \mathcal{A}} \sum_{b \in \mathcal{A},b\neq a} \E{\tau_{a}(T)\tau_{b}(T)}\\
 =& \frac{4}{T} \sum_{a \in \mathcal{A}} \sum_{b \in \mathcal{A},b\neq a} \left( n_a + (T- n) \bm{1}[a=\hat{a}^{*}]\right)
 \left( n_b +(T-n) \bm{1}[b=\hat{a}^{*}]\right)\\
=& \frac{4}{T} \sum_{a \in \mathcal{A}} \sum_{b \in \mathcal{A},b\neq a} ( n_a n_b  + n_b (T- n )  \bm{1}[a=\hat{a}^{*}] + n_a (T- n)    \bm{1}[b=\hat{a}^{*}])  \\
=& \frac{4}{T} \sum_{a \in \mathcal{A}} \sum_{b \in \mathcal{A},b\neq a} n_{a} n_{b} 
+  \frac{8(T-n)}{T} \sum_{b \in \mathcal{A},b\neq\hat{a}^*} \tau_b \\
<& \frac{4}{T} \left(n^2-\sum_{a\in\cA}n^2_a\right)
+  8n \leq 12n.
\end{align*}

Combining the above, and setting $\delta=1/T,$ we have (note that the maximal regret is $O(T),$ which would happen with probability at most $\delta=1/T$),
\begin{align}
\E{\tilde{R}_{\pi}(T)}\leq&  n (\Delta_{\max}+12) + (T-n) \varepsilon=O(n+(T-n)\varepsilon).
\end{align}
Recall that 
$n=\sum_{a\in\cA}n_a=\tilde{\Theta}\left({d^3}/{\varepsilon^2}\right),$ by setting $\varepsilon=\Theta(dT^{-1/3}),$ the statement follows.

\section{Proof of Proposition~\ref{lemma:phase_elimination_confidence_bound_theta_phi_any_t}}
\label{sec:proof_prop_phase_elimination_confidence_bound_theta_phi_any_t}
% Define $\alpha_{n}^{(4)}(\delta)=\sigma_{\max }^{2} \sqrt{d \log \left(\frac{n+\lambda}{\delta \lambda}\right)}+\lambda^{1 / 2}$.
 
\iffalse
\begin{lemma}[Theorem 2 in \cite{abbasi2011improved}]
For any $\delta > 0$, we have 
\begin{equation}
   \p{ \left\|\hat{\theta}_{(\ell)}-\theta_{*}\right\|_{V_{(\ell)}} \leq \sigma_{\max }^{2} \sqrt{d \log \left(\frac{T+\lambda}{\delta \lambda}\right)}+ \sqrt{\lambda}, ~ \forall \ell \in \mathbb{N}  } \geq 1-\delta. 
\end{equation}
\end{lemma}

By virtue of theorem 2 in \cite{abbasi2011improved}, for any $\delta > 0$, we have 
\begin{equation}
   \p{ \left\|\hat{\theta}_{(\ell)}-\theta_{*}\right\|_{V_{(\ell)}} \leq \sigma_{\max }^{2} \sqrt{d \log \left(\frac{T+\lambda}{\delta \lambda}\right)}+ \sqrt{\lambda}, ~ \forall \ell \in \mathbb{N}  } \geq 1-\delta. 
\end{equation}
\fi 

By virtue of Eq. (20.3) in \cite{lattimore2020bandit}, in phase $\ell$, for given $\delta_{\ell} > 0$ we have
\begin{equation}
   \p{ \left\|\hat{\theta}_{(\ell)}-\theta_{*}\right\|_{V_{(\ell)}} \leq 8 \sigma_{\max }^{2} \sqrt{d + \log \left(\frac{1}{\delta_{\ell} }\right)}  } \geq 1-\delta_{\ell}. 
\end{equation}
Choosing $\delta_{\ell} = \frac{\delta}{ 2 \ell^2 }$ and applying the union bound over $\ell \in \mathbb{N}$, we see that 

\begin{equation}
   \p{ \left\|\hat{\theta}_{(\ell)}-\theta_{*}\right\|_{V_{(\ell)}} \leq 8 \sigma_{\max }^{2} \sqrt{d + \log \left(\frac{2 T^2}{\delta }\right)}, ~ \forall \ell \in \mathbb{N}  } \geq 1-\delta. 
\end{equation}

Also, from theorem 1 of \cite{stay2019},
for any fixed $\delta > 0$, we have % and every $a\in\cA,$ 
\begin{equation}
\p{ \left\|\hat{\phi}_{(\ell)}-\phi_{*}\right\|_{V_{(\ell)}} \leq C_4    d\sqrt{\log(d)}  \log(\frac{T}{\delta })  , \forall \ell \in \mathbb{N} 
} \geq 1-\delta.
\end{equation}
Combining the above two concentration results we know that for given $\delta> 0$, with probability at least $1-\delta$, 
\begin{eqnarray}
\left | \innerprdct{ \rho \theta_{*} - \phi_{*} - \left( \rho \hat{\theta}_{(\ell)} - \hat{\phi}_{(\ell)} \right) , a } \right | 
&\leq& 
\left \|  \rho \theta_{*} - \phi_{*} - \left( \rho \hat{\theta}_{(\ell)} - \hat{\phi}_{(\ell)} \right) \right\|_{V_{(\ell)}} 
\left \| a \right\|_{V_{(\ell)}^{-1}} \nonumber \\
&\leq& \left (\rho \left \| \hat{\theta}_{(\ell)}-\theta_{*} \right \|_{V_{(\ell)}} + \left \| \hat{\phi}_{(\ell)}-\phi_{*} \right \|_{V_{(\ell)}} \right)  \left \| a \right \|_{V_{(\ell)}^{-1}} \nonumber \\
&\leq&  \left(  \rho   8 \sigma_{\max }^{2} \sqrt{d + \log \left(\frac{2 T^2 }{\delta }\right)} + C_4    d\sqrt{\log(d)}  \log(\frac{ T}{\delta })       \right)  \left \| a \right \|_{V_{(\ell)}^{-1}}    \nonumber \\ 
&\leq& \hat{C} d\sqrt{\log(d)} \log\left(\frac{ T}{\delta}\right) \left \| a \right\|_{V_{(\ell)}^{-1}}  \label{eq:bound_inner_product_MV_preliminary_1}  % \log\left(\frac{T+\lambda}{\delta \lambda}\right)
\end{eqnarray}
for any $\ell \in \mathbb{N}$.  
Applying the union bound over the action set $\mathcal{A}$, we arrive at 
\begin{equation}
    \p{ \left | \innerprdct{ \rho \theta_{*} - \phi_{*} - \left( \rho \hat{\theta}_{(\ell)} - \hat{\phi}_{(\ell)} \right) , a } \right | 
    \leq \hat{C} d\sqrt{\log(d)} \log\left(\frac{ K T}{\delta}\right) \left \| a \right\|_{V_{(\ell)}^{-1}}  , \forall \ell \in \mathbb{N} \text{ and } \forall a \in \mathcal{A}
} \geq 1-\delta.
\end{equation}

Recalling the definition of $n_{\ell,a}$ in \eqref{eq:phase_elimination_phase_length}, we have 
\begin{eqnarray*}
 V_{(\ell)}=\sum_{a \in \mathcal{A}_{\ell}} n_{\ell,a} a a^{\top} &=&  \sum_{a \in \mathcal{A}_{\ell}  } \left\lceil \hat{C}^2 \frac{d^{2} g_{\ell}(Q^{*}_{\ell}) \log(d) Q_{\ell}^{*}(a)}{\varepsilon_{\ell}^{2}} \log^{2} \left(\frac{ K T }{\delta}\right)\right\rceil a a^{\top} \\
 &\succeq& \hat{C}^{2} \frac{ d^{2} g_{\ell}(Q^{*}_{\ell}) \log(d)}{\varepsilon_{\ell}^{2}} \log^{2} \left(\frac{ K T}{\delta}\right) \sum_{a \in \mathcal{A}_{\ell} }  Q_{\ell}^{*}(a) a a^{\top}    .  %  \preceq
 % &=& \hat{C}^{2} \frac{ d^{2} g(Q^{*}_{\ell}) \log(d)}{\varepsilon_{\ell}^{2}} \log^{2} \left(\frac{ K T}{\delta}\right) \sum_{a \in \mathcal{A}_{\ell}} Q^{*}_{\ell} (a) a a^\top    % V( Q_{\ell}^{*})
\end{eqnarray*}

Hence, we see that 
\begin{eqnarray}
  \left \| a \right\|_{V_{(\ell)}^{-1}} &=& \sqrt{ a^{\top} V_{(\ell)}^{-1} a }  \leq \frac{\varepsilon_{\ell}^{}}{\hat{C} d \sqrt{\log{d}}} \frac{1}{ \log \left(\frac{ K T}{\delta}\right)  } \sqrt{\frac{a^{\top} \left(  \sum_{a \in \mathcal{A}_{\ell} }  Q_{\ell}^{*}(a) a a^{\top} \right)^{-1} a}{g_{\ell}(Q^{*}_{\ell}) }  } \nonumber  \\
 &\leq&   \frac{\varepsilon_{\ell}^{}}{\hat{C} d \sqrt{\log{d}}} \frac{1}{ \log \left(\frac{ K T}{\delta}\right)  }    \label{eq:bound_inner_product_MV_preliminary_2} ,
\end{eqnarray}
where the last inequality follows from the fact that $Q^{*}_{\ell}$ is an optimal solution to \eqref{eq:phase_elimination_g_optimal_design}. 
By combining \eqref{eq:bound_inner_product_MV_preliminary_1} and \eqref{eq:bound_inner_product_MV_preliminary_2}, we conclude the desired result. 




\section{Proof of Proposition~\ref{lemma:phase_elimination_pulled_times_upper_bound}}
\label{sec:proof_prop_phase_elimination_pulled_times_upper_bound}
We denote by $G_{\ell}^{a}$ the event that the MV estimate for action $a$ in phase $\ell$ deviates from the true value no more than $\varepsilon_{\ell}$, namely, 
$$
G_{\ell}^{a} = \left \{ \left| \innerprdct{\rho \hat{\theta}_{(\ell)} - \hat{\phi}_{(\ell)} - \left( \rho \theta_{*} - \phi_{*} \right), a } \right|  \leq \varepsilon_{\ell} \right \} .
$$
We say the \textit{good event} happens if for any action $a$ in exploration basis $\mathcal{A}_{\ell}$ in all phases, $G_{\ell}^{a}$ happens. I.e., we let 
$G = \underset{\ell}{\midcap} \underset{a \in \mathcal{A}_{\ell}}{\midcap} G_{a}^{\ell}$. 
By Lemma~\ref{lemma:phase_elimination_confidence_bound_theta_phi_any_t}, we know $G$ happens with probability at least $1 - \delta$. 

We first observe that if $G$ happens, then in phase $\ell$, the optimal action $a_{*}$ will not be eliminated at step (4) in Algorithm~\ref{algo:phase_ elimination}. 
To see this, suppose in phase $\ell$, the optimal arm $a_{*}$ were eliminated by some suboptimal action $b$, which would mean $\exists~b \in \mathcal{A}_{\ell}$ such that 
\begin{eqnarray}
&& 
\innerprdct{\rho \hat{\theta}_{(\ell)} - \hat{\phi}_{(\ell)}, b-a_{*}} > 2 \varepsilon_{\ell} \nonumber  \\
 &\Leftrightarrow~& 
\langle \rho \hat{\theta}_{(\ell)} - \hat{\phi}_{(\ell)}, b  \rangle - \varepsilon_{\ell} > 
\langle \rho \hat{\theta}_{(\ell)} - \hat{\phi}_{(\ell)}, a_*  \rangle + \varepsilon_{\ell}. \label{eq:good_estimate_1}
\end{eqnarray}
Since $G$ happens, we have 
$$
\langle \rho \theta_{*} - \phi_{*}, b  \rangle \geq \langle \rho \hat{\theta}_{(\ell)} - \hat{\phi}_{(\ell)}, b  \rangle - \varepsilon_{\ell}  ~~\text{and}~~ \langle \rho \hat{\theta}_{(\ell)} - \hat{\phi}_{(\ell)}, a_*  \rangle + \varepsilon_{\ell} \geq \langle \rho \theta_{*} - \phi_{*}, a_*  \rangle
,$$
which, combined with \eqref{eq:good_estimate_1}, leads to the contradiction $\langle \rho \theta_{*} - \phi_{*}, b  \rangle >\langle \rho \theta_{*} - \phi_{*}, a_*  \rangle$.

%Next, we argue that when $G$ happens, the loss in stage $\ell$ from pulling an arm once is at most a constant times $\varepsilon_{\ell}$. 
Next, we argue that provided the good event $G$ happens, a suboptimal arm $a$ with gap $\Delta_a$ will be eliminated before $\ell_a = \min \{\ell: 2 \varepsilon_\ell < \Delta_a \}$. 
Indeed, at step (3) of phase $\ell+1$, the estimated MV gap of action $a$ based on estimators in the previous phase $\ell$ is no more than  $2 \varepsilon_\ell$, i.e., 
$$
\max _{b \in \mathcal{A}_{\ell+1 }} \innerprdct{ \rho \hat{\theta}_{(\ell)} - \hat{\phi}_{(\ell)}, b-a } \leq 2 \varepsilon_{\ell} = 4 \varepsilon_{l+1}.
$$
In particular, the optimal action $a_*$ remains in $\mathcal{A}_{\ell+1}$. Hence, we have 
\begin{equation} \label{eq:1}
    \innerprdct{ \rho \hat{\theta}_{(\ell)} - \hat{\phi}_{(\ell)} , a_* - a } \leq 2 \varepsilon_{\ell}
\end{equation}
for any suboptimal arm $a \in \mathcal{A}_{\ell+1}$.
On the other hand, the event $G$ implies that 
$-\varepsilon_{\ell}   \leq \innerprdct{ \rho \hat{\theta}_{(\ell)} - \hat{\phi}_{(\ell)} - \left( \rho \theta_{*} - \phi_{*} \right) , a  } \leq \varepsilon_{\ell}$ 
and $-\varepsilon_{\ell} \leq \innerprdct{  \rho \hat{\theta}_{(\ell)} - \hat{\phi}_{(\ell)} - \left( \rho \theta_{*} - \phi_{*} \right), a_*  } \leq \varepsilon_{\ell}$ hold, which means    
% $$
% - 2\varepsilon_{\ell} \leq \innerprdct{  \rho \hat{\theta}_{(\ell)} - \hat{\phi}_{(\ell)} - \left( \rho \theta_{*} - \phi_{*} \right) , a_* - a  } \leq % 2\varepsilon_{\ell},
% $$
% which is equivalent to 
\begin{equation} \label{eq:2}
  -2\varepsilon_{\ell} \leq 
\innerprdct{ \rho \theta_{*} - \phi_{*}  , a_* - a  } 
- \innerprdct{ \rho \hat{\theta}_{(\ell)} - \hat{\phi}_{(\ell)} , a_* - a  }
\leq 2\varepsilon_{\ell}. 
\end{equation}
Combining \eqref{eq:1} and \eqref{eq:2} yields that 
$$
\Delta_a = \innerprdct{ \rho \theta_{*} - \phi_{*}  , a_* - a } \leq 4 \varepsilon_{\ell} = 2 \varepsilon_{\ell+1}.
$$
Therefore, the true MV gap incurred by a suboptimal action in $\mathcal{A}_{\ell}$ is at most $2 \varepsilon_\ell$.
% is at most $T_{\ell} \cdot 2 \varepsilon_{\ell}$. 
In other words, when $G$ happens, a suboptimal action $a$ with gap $\Delta_a$ will be eliminated before phase $\ell_a = \min \{\ell \geq 1: 2 \varepsilon_\ell < \Delta_a  \} = \lceil \log_2(2 / \Delta_a ) \rceil$. This also indicates 
\begin{align}\label{eq:eps_delta}
\varepsilon_{\ell_a}\geq\frac{\Delta_a}{4}\,.
\end{align}

By setting $\delta = {1}/{ T}$, we can therefore bound the quantity $\E{\tau_a(T)} $:
\begin{eqnarray}
\E{\tau_a(T)} &\leq&  \frac{1}{T} \cdot T  + (1-\frac{1}{T}) \sum_{\ell=1}^{\ell_a} n_{\ell,a} \nonumber \\ 
&\leq& 1 + \sum_{\ell=1}^{\ell_a} \left\lceil \hat{C}^2 \frac{d^{2} g_{\ell}(Q_{\ell}^{*}) \log(d) Q_{\ell}^{*} (a) }{\varepsilon_{\ell}^{2}} \log^2 \left(\frac{ K T }{\delta}\right)\right\rceil \\
&\leq& 1 + \sum_{\ell=1}^{\ell_a} \left( \hat{C}^2 \frac{d^{3}  \log(d) Q^{*}_{\ell} (a)}{\varepsilon_{\ell}^{2}} \log^{2} \left(\frac{ K T^{} }{\delta}\right) + 1 \right)  \nonumber \\
&\leq& 1 +  \hat{C}^{2} d^{3} \log(d) \log^2(K T^{2}) \sum_{\ell=1}^{\ell_a}  \frac{Q^*_{l}(a)}{\varepsilon_\ell^{2}}  + \ell_a  \nonumber\\ 
&\leq& 1 +  \hat{C}^{2} d^{3} \log(d) \log^2(K T^{2})  \frac{\sum_{\ell=1}^{\ell_a}  Q^*_{l}(a)}{\varepsilon_{\ell_a}^{2}}  + \log \left( \frac{2}{\Delta_a} \right) + 1  \nonumber \\
&\leq& 2 +  \frac{16\hat{C}^{2} d^{3} \log(d) \log^2(K T^{2})}{\Delta^2_a}  \left(\sum_{\ell=1}^{\ell_a}  Q^*_{l}(a)\right)  +  \log \left( \frac{2}{\Delta_a} \right) \,.  \nonumber 
%&=& O\left(  \frac{d^{3} \log(d)   \log^2(K T) } {\Delta_a^2 }  + \log({\Delta_a}^{-1}) \right) .
\end{eqnarray}
Here, the second last inequality uses the fact that $\epsilon_{l-1}>\epsilon_l$ and the last step uses \eqref{eq:eps_delta}.
Therefore, noting the simple algebraic fact that $\log \left( 2 / \Delta \right) <  1/\Delta^2$ for positive $\Delta$, we conclude that 
$$
\E{\tau_a(T)} \leq  O \left(  \frac{ d^{3} \log(d) \log^2(K T)}{\Delta^2_a}  \left( \sum_{\ell=1}^{\ell_a}  Q^*_{l}(a) \right)   \right) . 
$$

% \Jingwei{In the last two lines, $\log({\Delta_a}^{-1})$ should be $\lceil \log_2(2 / \Delta_a ) \rceil$? Shall we also include this term in Eq. 28?   }
% \Ruihao{Oh yes, please change them to $\lceil \log_2(2 / \Delta_a ) \rceil$ if needed. We do not need to include this, it appears to me that $\log(\Delta^{-1})$ is dominated by $1/\Delta^2$?}
% \Jingwei{Yes. $\log \left( \frac{2}{\Delta} \right) <  1/\Delta^2$ for positive $\Delta$. I checked using $Plot[Log[2/x] - 1/x^2, {x, 0, 100}]$ in Mathematica. But I have a very basic question of whether we should report$ \E{\tau_a(T)} \leq  O \left(  \frac{ d^{3} \log(d) \log^2(K T^{2})}{\Delta^2_a}  \left( \sum_{\ell=1}^{\ell_a}  Q^*_{l}(a) \right)    \right) $ or $ \E{\tau_a(T)} \leq  O \left(  \frac{ d^{3} \log(d) \log^2(K T^{2})}{\Delta^2_a}  \left( \sum_{\ell=1}^{\ell_a}  Q^*_{l}(a) \right)   + \log \left( \frac{1}{\Delta_a} \right) \right) $. Because we have to sum over $K$, if we do the latter, we will have a $\sum_{a \in \mathcal{A}} \log( 1 / \Delta_a )$ in the bound on the regret, which is linear in $K$. If we do the former, the $K$ dependence on the proxy regret would be only of $\log(K)$. Now I kept the latter one. } \Ruihao{You would only have this term for those who has $Q^*_l(a)\geq 0\,.$ So remove this.}
\iffalse


\begin{equation} \label{eq:phase_elimination_phase_length}
    n_{\ell,a}=\left\lceil \hat{C}^2 \frac{d^{2} g_{\ell}(Q_{\ell}^{*}) \log(d) Q_{\ell}^{*} (a) }{\varepsilon_{\ell}^{2}} \log^2 \left(\frac{ K T }{\delta}\right)\right\rceil 
\end{equation}

By setting $\delta = \frac{1}{ T}$, we can therefore bound the quantity $\E{\tau_a(T)} $:
\begin{eqnarray}
\E{\tau_a(T)} &\leq&  \frac{1}{T} \cdot T  + (1-\frac{1}{T}) \sum_{\ell=1}^{\ell_a} n_{\ell,a} \nonumber \\ 
&\leq& 1 + \sum_{\ell=1}^{\ell_a} n_{(\ell)} \\
&\leq& 1 + \sum_{\ell=1}^{\ell_a} \left( \hat{C}^2 \frac{d^{3}  \log(d) Q^{*}_{\ell} (a)}{\varepsilon_{\ell}^{2}} \log^{2} \left(\frac{ K T^{} }{\delta}\right) + \frac{d(d+1)}{2} \right)  \nonumber \\
&=& 1 +  \hat{C}^{2} d^{3} \log(d) \log^2(K T^{2}) \sum_{\ell=1}^{\ell_a}  \frac{1}{\varepsilon_\ell^{2}}  + \ell_a \cdot \frac{d(d+1)}{2} \nonumber \\
&=& O\left(  \frac{d^{3} \log(d)   \log^2(K T^2) } {\Delta_a^2 }  + d^2\log(\frac{1}{\Delta_a}) \right) .
\end{eqnarray}

\fi 



\end{APPENDIX}
